# Supplementary material for: TBP-Former: Learning Temporal Bird's-Eye-View Pyramid for Joint Perception and Prediction in Vision-Centric Autonomous Driving
Source: arXiv:2303.09998 source file (2023-03-22)
Supplement: Supplementary file 1 [file supp.tex]

\section*{Appendix}

\section*{A. Results on BEV Detection task}

The BEV representations could be constructed from our proposed modules (PoseSync Encoder and STPT). Then we use CenterPoint's~\cite{yin2021center} detection head for object detection. To compare TBP-Former and previous methods, we calculate vehicles' Average Precision under BEV (APBEV) at different thresholds. Table~\ref{supp:detection} shows that our method achieves comparable results compared with others. 

\begin{table}[h]
\scriptsize
\centering
\begin{tabular}{c|c|ccc}
\toprule
Methods         & \begin{tabular}[c]{@{}c@{}}Input RGB \\ Resolution\end{tabular} & AP@0.3 & AP@0.5 & AP@0.7 \\
\hline
\hline
BEVFormer-small~\cite{bevformer} & 1280 $\times$ 720             & 55.42     & 35.76     & 13.13     \\
BEVFormer-base~\cite{bevformer}  & 1600 $\times$ 900             & 56.94     & 40.40     & 16.38     \\
BEVerse~\cite{beverse}         & 1408 $\times$ 512             & 54.30     & 37.86     & 16.12     \\ \hline
Ours            & 480 $\times$ 224              & 55.43     & 38.49     & 17.98    \\
\bottomrule
\end{tabular}
\caption{Detection results on nuScenes validation dataset.}
\label{supp:detection}
\end{table}

\section*{B. Number of Parameters and Inference Time}

 Table~\ref{supp:temporal_ablation} shows the parameter numbers of different temporal models and their inference times. TBP-Former is the most parameter-efficient model with top performance and leading speed. 

\begin{table}[ht]
\scriptsize
\centering
\begin{tabular}{c|cc|ccc}
\toprule
Methods & IoU & VPQ & \# param. & FPS & Inference Time\\ \hline
\hline
$\text{MotionNet}^{\dag}$ & 35.4 & 30.6 & 11.26M & 3.84 & 22ms \\
$\text{FIERY}^{\dag}$ & 38.3 & 32.1 & 12.37M & 2.69 & 134ms \\
$\text{BEVerse}^{\dag}$ & 40.2 & 34.0 & 13.17M & 1.78 & 322ms \\ \hline
TBP-Former & 41.9 & 36.9 & 9.42M & 2.44 & 165ms \\ \hline
\end{tabular}
\caption{The number of parameters and inference time for prediction models. \dag: We use MotionNet, FIERY, and BEVerse's temporal models to replace our proposed STPT. }
\label{supp:temporal_ablation}
\end{table}

\section*{C. Ablation Experiments on STPT}

Table~\ref{supp:stpt_layers} compares our method's performance on PnP task with different pyramid layers. We ended up with a 4-layer encoder-decoder architecture. 

\begin{table}[h]
\centering
\begin{tabular}{c|cccc}
\toprule
\begin{tabular}[c]{@{}c@{}}\# Pyramid \\ Layers\end{tabular}                                                   & IoU-S                            & VPQ-S                           & IoU-L                            & VPQ-L                           \\ \hline
\hline
1   & 64.30                           & 41.93                           & 56.44                           & 37.35                           \\
2               & 64.36                           & 42.1                           & 56.53                           & 37.57                           \\
3           & 64.30                           & 41.94                           & 56.45                           & 37.37                           \\ \hline
4                                                             & \textbf{64.61} & \textbf{42.31} & 56.44 & 37.50 \\ \hline
\end{tabular}
\caption{Ablation experiment of pyramid layers of STPT. -S represents short range (30m $\times$ 30m) and -L represnets long range (100m $\times$ 100m). }
\label{supp:stpt_layers}
\end{table}

\section*{D. Visualization of STPT}
To better understand the function of STPT, we visualize the attention matrix of the first layer of STPT's encoder. As is shown in Fig.~\ref{fig:supp_stpt}, our model can locate and track the moving vehicles in historical frames, which is beneficial for future states prediction. 

\begin{figure}[htb]
    \centering
    \includegraphics[scale=0.4]{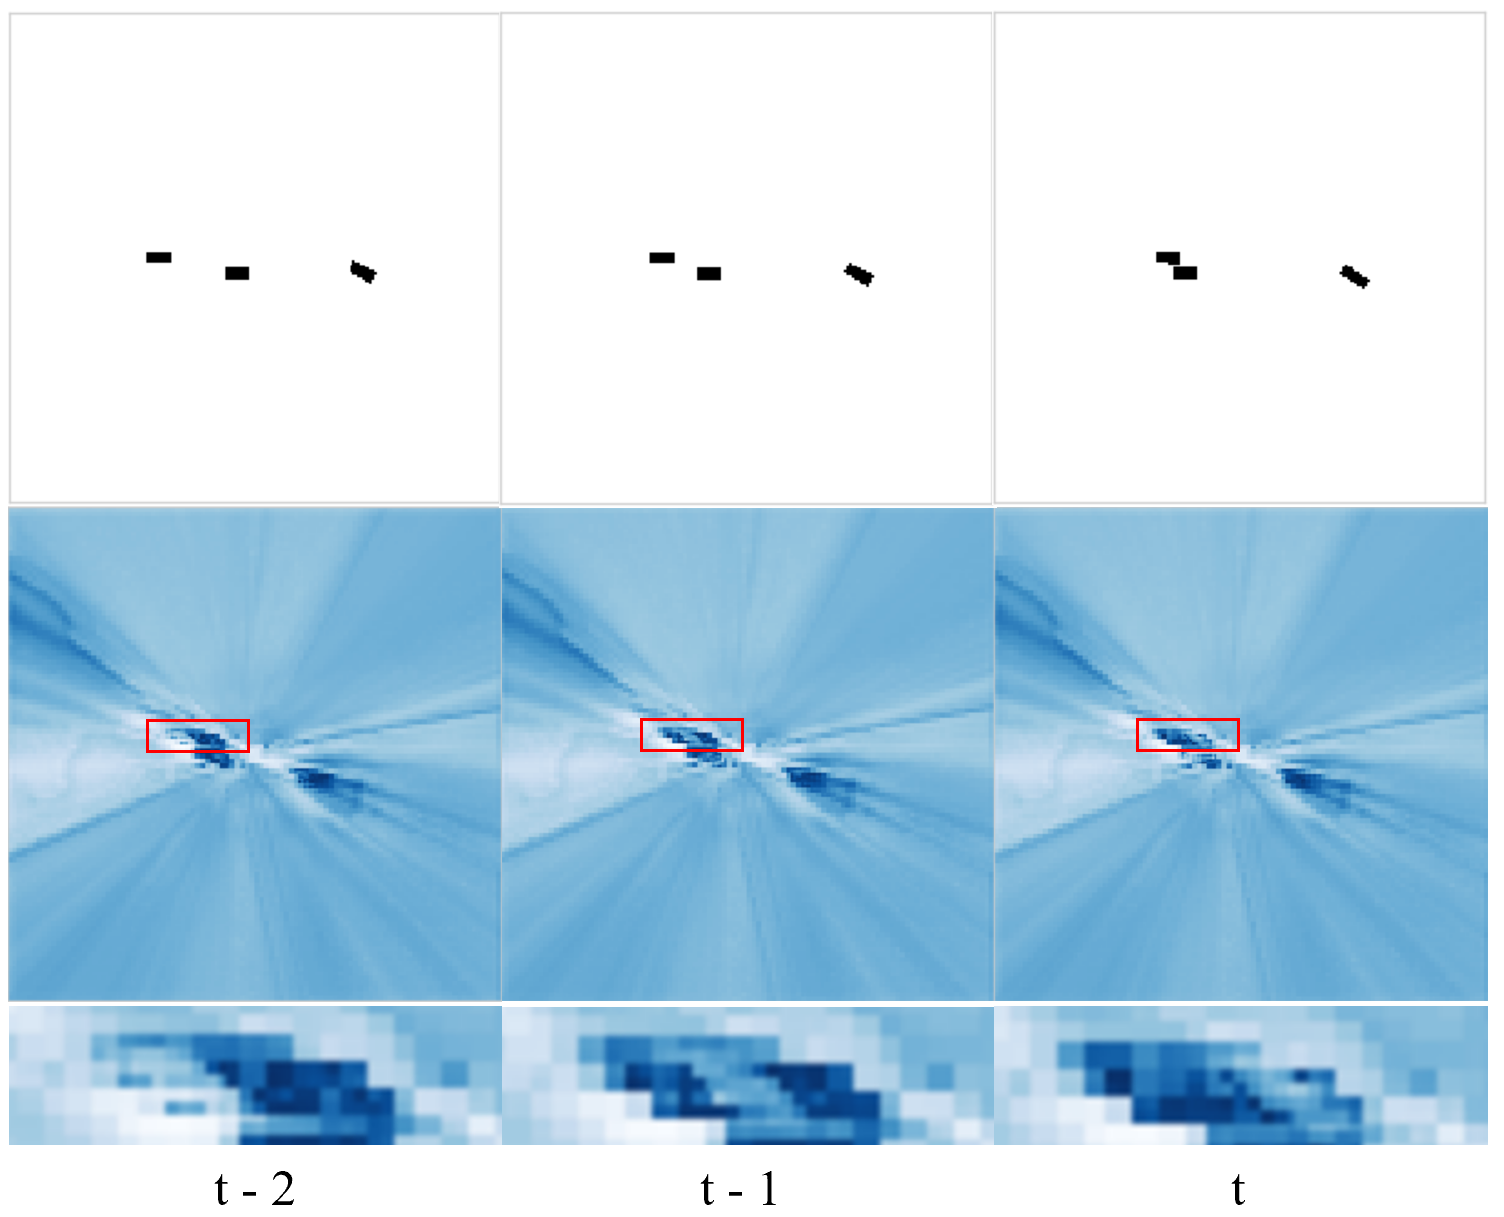}
    \caption{Visualization of attention matrix calculated by STPT. }
    \label{fig:supp_stpt}
\end{figure} 

\begin{figure*}[htb]
    \centering
    \includegraphics[scale=1.4]{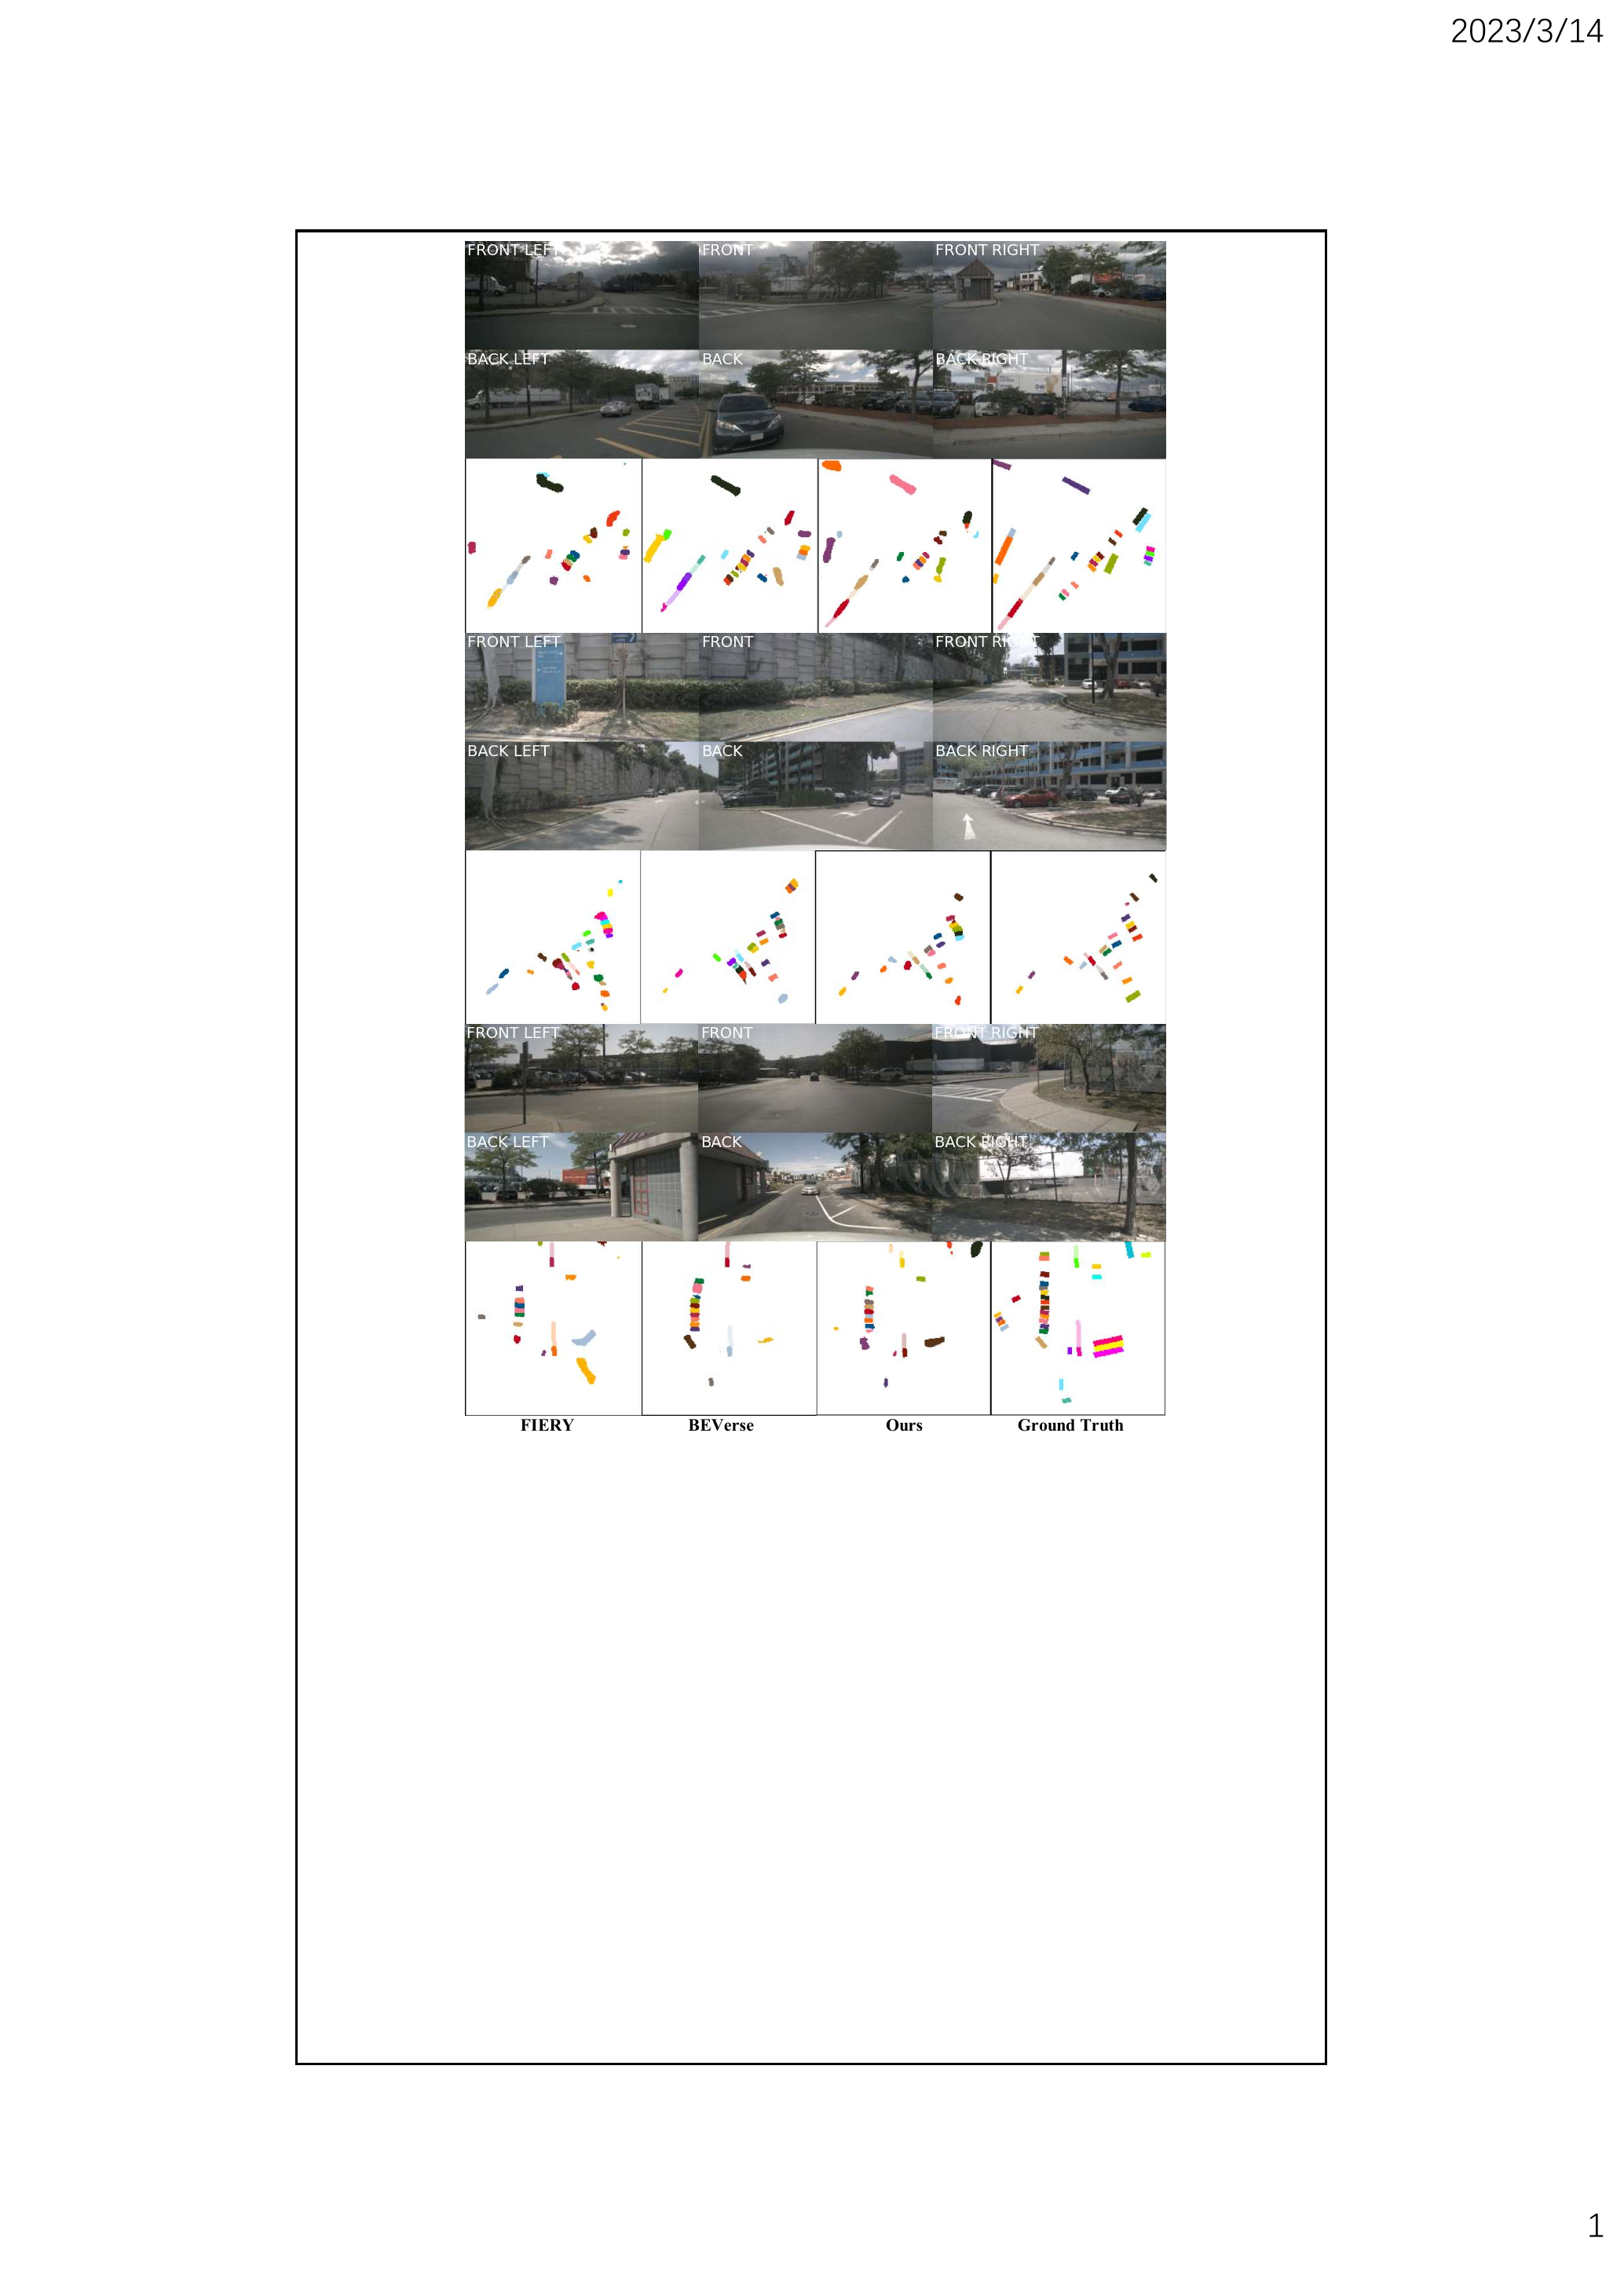}
    \caption{Comparisons between our method and previous methods. }
    \label{fig:supp_compare}
\end{figure*}
